# Supplementary material for: Quantum droplets with magnetic vortices in spinor dipolar Bose-Einstein condensates
Source: arXiv:2402.18885 ancillary file (2024-02-29)
Supplement: Supplementary file 1 [file supplement.pdf]

# Quantum droplets with magnetic vortices in spinor dipolar Bose-Einstein condensates

Shaoxiong Li and Hiroki Saito
*Department of Engineering Science, University of Electro-Communications, Tokyo 182-8585, Japan*

## I. MAGNETIC MOMENT OF A EUROPIUM ATOM

The magnetic moment of an atom with hyperfine spin $F$, total electron spin $S$, and nuclear spin $I$ with orbital angular momentum $L = 0$ is given by $\mu = g\mu_B F$ with the $g$ factor [1]

$$g = \frac{F(F+1) + S(S+1) - I(I+1)}{F(F+1)}. \tag{S1}$$

For the electronic ground state of $^{151}$Eu (and also $^{153}$Eu), $S = 7/2$ and $I = 5/2$. The magnetic moment $\mu$ and the dipolar length $a_{\rm dd} = \mu_0\mu^2 M/(12\pi\hbar^2)$ of $^{151}$Eu are given in Table S1.

| $F$ | 1 | 2 | 3 | 4 | 5 | 6 |
|---|---|---|---|---|---|---|
| $\mu/\mu_B$ | 9/2 | 13/3 | 19/4 | 27/5 | 37/6 | 7 |
| $a_{dd}/a_B$ | 24.72 | 22.92 | 27.54 | 35.60 | 46.42 | 59.82 |

TABLE S1. Magnetic moment $\mu$, in units of the Bohr magneton $\mu_B$, and the dipolar lengths $a_{dd}$, in units of the Bohr radius $a_B$, for $^{151}$Eu with hyperfine spin $F$.

## II. DERIVATION OF THE VARIATIONAL ENERGY

To analyze the torus-shaped droplet state with a spin vortex, we use the following variational wave function (Eq. (2) in the main text)

$$\mathbf{\Psi}_v(\boldsymbol{r}) = \sqrt{\rho_v(r,z)}\, e^{-iS_z\phi}\boldsymbol{\zeta}^{(y)}, \tag{S2}$$

where the density distribution $\rho_v(r,z)$ is given by (Eq. (3) in the main text)

$$\rho(r,z) = \frac{N}{\pi^{3/2}\sigma_r^{2\lambda+2}\sigma_z\Gamma(\lambda+1)} r^\lambda e^{-\frac{r^2}{\sigma_r^2}-\frac{z^2}{\sigma_z^2}}. \tag{S3}$$

Substituting Eqs. (S2) and (S3) into the kinetic energy $E_{\rm kin}$, we obtain

$$\begin{aligned} E_{\rm kin} &= \frac{\hbar^2}{2M}\int d\boldsymbol{r}\left[(\nabla\sqrt{\rho_v})^2 + \frac{F}{2r^2}\rho_v\right] \\ &= \frac{N\hbar^2}{2M}\left[\frac{1}{2\sigma_r^2}\left(2+\frac{F}{\lambda}\right) + \frac{1}{2\sigma_z^2}\right], \end{aligned} \tag{S4}$$

where the term proportional to $F$ arises from the winding of the spin vector. For the present form of the variational wave function, the $z$ component of the magnetization $f_z(\boldsymbol{r})$ vanishes and the integral part $I$ of the DDI energy $E_{\rm ddi}$ can be expressed as

$$\begin{aligned} I &= \int \frac{d\boldsymbol{r}d\boldsymbol{r}'}{|\boldsymbol{r}-\boldsymbol{r}'|^3}\left\{\boldsymbol{f}(\boldsymbol{r})\cdot\boldsymbol{f}(\boldsymbol{r}') - 3[\boldsymbol{f}(\boldsymbol{r})\cdot\boldsymbol{e}][\boldsymbol{f}(\boldsymbol{r}')\cdot\boldsymbol{e}]\right\} \\ &= \int \frac{d\boldsymbol{r}d\boldsymbol{r}'}{|\boldsymbol{r}-\boldsymbol{r}'|^3}\bigg\{-\frac{1}{2}f_+(\boldsymbol{r})f_-(\boldsymbol{r}')(1-3e_z^2) \\ &\quad -\frac{3}{4}\left[f_+(\boldsymbol{r})f_+(\boldsymbol{r}')e_-^2 + f_-(\boldsymbol{r})f_-(\boldsymbol{r}')e_+^2\right]\bigg\} \\ &= \int\frac{d\boldsymbol{k}}{(2\pi)^3}\bigg\{\frac{2\pi}{3}(1-3\cos^2\alpha)\tilde{f}_+(-\boldsymbol{k})\tilde{f}_-(\boldsymbol{k}) \\ &\quad +\pi\sin^2\alpha\left[e^{-2i\beta}\tilde{f}_+(-\boldsymbol{k})\tilde{f}_+(\boldsymbol{k}) + e^{2i\beta}\tilde{f}_-(-\boldsymbol{k})\tilde{f}_-(\boldsymbol{k})\right]\bigg\}, \end{aligned} \tag{S5}$$

where $\alpha$ and $\beta$ are the polar and azimuthal angles in the $\boldsymbol{k}$-space, respectively, $\tilde{f}_\pm(\boldsymbol{k})$ is the Fourier transform of $f_\pm(\boldsymbol{r}) = f_x(\boldsymbol{r}) \pm i f_y(\boldsymbol{r})$, and the convolution theorem was used in the third equality. Noting that $\tilde{f}_\pm(\boldsymbol{k})$ is proportional to $\pm e^{\pm i\beta}$ and $\tilde{f}_\pm(-\boldsymbol{k}) = -\tilde{f}_\pm(\boldsymbol{k})$ for the forms of Eqs. (S2) and (S3), Eq. (S5) can be reduced to

$$\begin{aligned} I &= -\frac{4\pi}{3}\int\frac{d\boldsymbol{k}}{(2\pi)^3}|\tilde{f}_+(\boldsymbol{k})|^2. \\ &= -\frac{4\pi F^2}{3}\int d\boldsymbol{r}\rho^2(\boldsymbol{r}). \end{aligned} \tag{S6}$$

This result indicates that $E_{\rm ddi}/E_s = -\varepsilon_{\rm dd}$, and therefore $\varepsilon_{\rm dd} > 1$ is the necessary condition for the droplet to be bound by the attractive part of the DDI. The DDI and $s$-wave interaction energies are calculated to be

$$\frac{ME_{\rm ddi}}{N\hbar^2} = -\varepsilon_{\rm dd}\frac{ME_s}{N\hbar^2} = -\frac{Na_{\rm dd}\Gamma(\lambda+1/2)}{\sqrt{2}\pi\Gamma(\lambda+1)\sigma_r^2\sigma_z}. \tag{S7}$$

The LHY energy in Eq. (1) in the main text is obtained as

$$\frac{ME_{\rm LHY}}{N\hbar^2} = \frac{2^{(5\lambda+17)/2}N^{3/2}a^{5/2}\lambda\Gamma(5\lambda/2)\chi(\varepsilon_{\rm dd})}{3\pi^{7/4}5^{(5\lambda+3)/2}\Gamma^{5/2}(\lambda+1)\sigma_r^3\sigma_z^{3/2}}. \tag{S8}$$

The variational energy is given by the sum of these energies,

$$E = E_{\rm kin} + E_s + E_{\rm ddi} + E_{\rm LHY}. \tag{S9}$$

## III. $\varepsilon_{\rm dd}$ AND $N$ DEPENDENCE OF THE VARIATIONAL PARAMETERS

Figure S1 shows the variational parameters that minimize the variational energy. The droplet size $\sigma_r$ (also

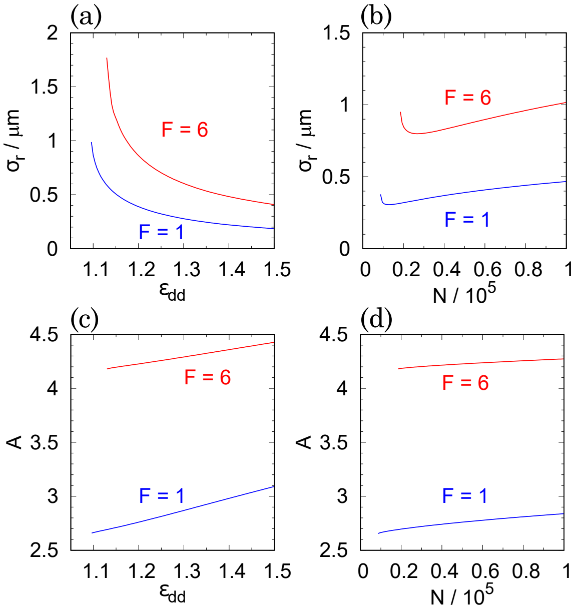


FIG. S1. $\varepsilon_{\rm dd}$ and $N$ dependence of the variational parameters that minimize the variational energy. (a) Dependence of $\sigma_r$ on $\varepsilon_{\rm dd}$, (b) $\sigma_r$ on $N$, (c) $A$ on $\varepsilon_{\rm dd}$, and (d) $A$ on $N$ for $F = 1$ and 6. $N = 50000$ in (a) and (c), and $\varepsilon_{\rm dd} = 1.2$ in (b) and (d).

$\sigma_z$) decreases with $\varepsilon_{\rm dd}$ due to the attractive nature of the DDI, as shown in Fig. S1(a), while $\sigma_r$ increases with $N$ except near the critical number of atoms, as shown in Fig. S1(b). In Figs. S1(a) and S1(b), the droplet size steeply increases near the critical values (left-hand edges of the lines), since the droplet is about to unbound. Figure S1(c) shows the aspect ratio $A(\lambda)$ of the torus defined by

$$A(\lambda) = \frac{\langle r \rangle}{\sqrt{\langle r^2 \rangle - \langle r \rangle^2}} = \left[ \frac{(\lambda+1)\Gamma^2(\lambda+1)}{\Gamma^2(\lambda+3/2)} - 1 \right]^{-1/2}, \tag{S10}$$

where $\langle \cdots \rangle$ represents the expectation value with respect to the variational wave function. The aspect ratio $A(\lambda)$ in Eq. (S10) is a monotonically increasing function of $\lambda$. We find from Figs. S1(c) and S1(d) that $A(\lambda)$ is largely dependent on the spin $F$. This is due to the term proportional to $F/\lambda$ in Eq. (S4), i.e., the kinetic energy arising from the spin winding. The aspect ratio is not significantly sensitive to $\varepsilon_{\rm dd}$ or $N$, as shown in Figs. S1(c) and S1(d). These tendencies are in agreement with the result in Fig. 1(d) in the main text, obtained by the imaginary-time evolution of the Gross-Pitaevskii equation.


[1] L. D. Landau and E. M. Lifshitz, *Quantum Mechanics*, 3rd ed., Sec. 121 (Butterworth-Heinemann, Oxford, 1981).
